# Supplementary material for: DepreSym: A Depression Symptom Annotated Corpus and the Role of LLMs as Assessors of Psychological Markers
Source: arXiv:2308.10758 source file (2023-08-21)
Supplement: Supplementary file 1 [file A-_Appendix.tex]

\begin{appendix}
\section{Guidelines}

Both the human annotators and the LLMs (ChatGPT and GPT-4) were provided with the following guidelines to make the annotation process comparable:

\em

Given the folllowing instructions:

Assume you are given a BDI item, e.g.: \\
15. Loss of Energy \\
 -I have as much energy as ever. \\
 -I have less energy than I used to have. \\
 -I don't have enough energy to do very much. \\
 -I don't have enough energy to do anything. 

The task consists of annotate sentences in the collection that are topically-relevant to the item (related to the question and/or to the answers).

Note: A relevant sentence should provide some information about the state of the own writer related to the topic of the BDI item. But it is not necessary that the exact same words are used.

Your job is to assess sentences on how topically-relevant they are for a concrete BDI item.

The relevance grades are: \\
1. Relevant: A relevant sentence should be topically-related to the BDI-item (regardless of the wording) and, additionally, it should refer to the state of the writer about the BDI-item. \\
0. Non-relevant: A non-relevant sentence does not address any topic related to the question and/or the answers of the BDI-item (or it is related to the topic but does not represent the writer's state about the BDI-item). For example, for BDI-item 15, a sentence that does not talk about the individual’s level of energy (regardless of the wording), then is a non-relevant sentence. 

Examples (assessment of sentences ranked for BDI-item number 15): \\
“I cannot control my energy these days”: Relevant \\
“My sister has no energy at all”: Non-relevant sentence (because it does not refer to the writer who posted this sentence) \\
“The book was about a highly energetic man”: Non-relevant sentence (because it does not refer to the writer who posted this sentence) \\
“I feel more tired than usual”: Relevant \\
“The football team is named Top Energy”: Non-relevant \\
“I am totally lonely”: Non-relevant (it does not mention energy) \\
“I've just recharged my batteries”: Relevant \\
“I am lost”: Non-relevant

For the the BDI item X. Could you annotate the following sentences for relevance to the item (and only for that item):

\end{appendix}
